# Supplementary material for: The influence of high-energy local orbitals and electron-phonon interactions on the band gaps and optical spectra of hexagonal boron nitride
Source: arXiv:2003.12704 source file (2020-05-24)
Supplement: Supplementary file 1 [file supplemental.pdf]

# Supplemental Material for "The influence of high-energy local orbitals and electron-phonon interactions on the band gaps and optical spectra of hexagonal boron nitride"

Tong Shen,[1] Xiao-Wei Zhang,[2,*] Honghui Shang,[3] Min-Ye Zhang,[4]
Xinqiang Wang,[1,5] En-Ge Wang,[2,6,7] Hong Jiang,[8,†] and Xin-Zheng Li[1,9,‡]

[1]*State Key Laboratory for Artificial Microstructure and Mesoscopic Physics, Frontier Science Center for Nano-optoelectronics and School of Physics, Peking University, Beijing, China*
[2]*International Center for Quantum Materials and School of Physics, Peking University, Beijing, China*
[3]*State Key Laboratory of Computer Architecture, Institute of Computing Technology, Chinese Academy of Sciences, Beijing, China*
[4]*Beijing National Laboratory for Molecular Sciences, College of Chemistry and Molecular Engineering, Peking University, Beijing,China*
[5]*Collaborative Innovation Center of Quantum Matter, Peking University, Beijing 100871, P. R. China*
[6]*Ceramic Division, Songshan Lake Lab, Institute of Physics, Chinese Academy of Sciences, Guangdong, China*
[7]*School of Physics, Liaoning University, Shenyang, China*
[8]*Beijing National Laboratory for Molecular Sciences, College of Chemistry and Molecular Engineering, Peking University, Beijing, China*
[9]*Collaborative Innovation Center of Quantum Matter, Peking University, Beijing, China*

(Dated: May 24, 2020)

* willzxw@pku.edu.cn
† jianghchem@pku.edu.cn
‡ xzli@pku.edu.cn

# I. VAN DER WAALS INTERACTIONS

In layered materials, the van der Waals (vdW) interactions are often important in describing the inter-layer distances. In all our calculations, however, we have not used the structures given by the vdW functionals. Experimental lattice constants were used. The reasons are twofold. First, for quasiparticles, the use of experimental lattice constants is a convention in *GW* and BSE calculations in order to eliminate the effects of the uncertainties given by structure parameters on band gaps [see e.g. Refs. 23, 26, 28-36 of the manuscript]. This is appropriate and, in fact, necessary because one likes to compare our theoretical results with experimental band gaps without unwanted problems caused by differences in the lattice constants. Second, for electron-phonon calculations, the structure optimizations are usually needed for phonon calculations. However, we found that the structure-optimizations could be problematic. This is shown in Table S1. The PBE functional gives a much larger lattice constant $c$ than the experimental one. While LDA, PBE+optB86b, and SCAN give the smallest direct band gap at the k-point M instead of at H. These are clearly inconsistent with our understandings of $h$-BN. Using experimental structure, on the other hand, eliminates all these problems and one does not get imaginary mode in the phonon calculations either. Therefore, we also use the experimental structure to do calculations for electron-phonon interactions.

TABLE S1. The experimental lattice constant and geometry-optimized lattice constants using different functionals, e.g. LDA, PBE, PBE+optB86b for vdW-corrections, and SCAN.

| | Without geometry optimization | | With geometry optimization | | | |
|---|---|---|---|---|---|---|
| lattice parameter | Exp. | | LDA | PBE | PBE+optB86b | SCAN |
| a | 2.504 | | 2.491 | 2.513 | 2.513 | 2.496 |
| c | 6.661 | | 6.430 | 7.924 | 6.464 | 6.721 |
| bandgap | LDA | PBE | LDA | PBE | PBE | SCAN |
| Direct(at H) | 4.497 | 4.635 | 4.525 | 4.64 | 4.600 | 4.788 |
| Direct(at M) | 4.517 | 4.711 | 4.427 | 5.239 | 4.570 | 4.751 |
| Fundamental ($T_1 - M$) | 4.033 | 4.229 | 3.991 | 4.503 | 4.154 | 4.237 |

# II. OPTICAL SPECTRUM

## A. Imaginary parts of dielectric functions in RPA and BSE level

The electron-hole interactions drag the absorption edge to lower frequency and increase the overlap between the wavefunctions of the electrons and holes. This changes the line-shape of the absorption spectrum, and results in larger absorption strength in the low-frequency spectrum edge in the BSE calculation than that of the RPA one. This is a feature in common for most materials. The only difference here is that the exciton energy in $h$-BN is order of magnitude larger than most other semiconductors, e.g. Si, and this effect is much more apparent. This is not in conflict with the $f$-sum rule, since the rule is written as

$$\int \omega\epsilon_2(\omega) = \frac{2\pi^2 e^2 n}{m}. \quad (1)$$

where $n$ is the electron density and $m$ is the electron mass. For this formula, there are two points to stress: 1) the integral function is the imaginary part of the dielectric function multiplied by the frequency and $\epsilon_2(\omega)$ at higher frequency has a larger weight; 2) the integral is over the whole frequency range and one cannot investigate the f-sum rule in terms of the spectra over a small frequency range. Besides, although the electron-hole interactions enhance the absorption, the spectra have a large redshift with respect to the one of RPA as shown in Fig. S1. In the end, to clarify the question numerically, we calculate the integral up to 20 eV using the imaginary parts of dielectric functions in BSE and RPA level. The results are 294 $(\text{eV})^2$ for BSE and 292 $(\text{eV})^2$ for RPA.

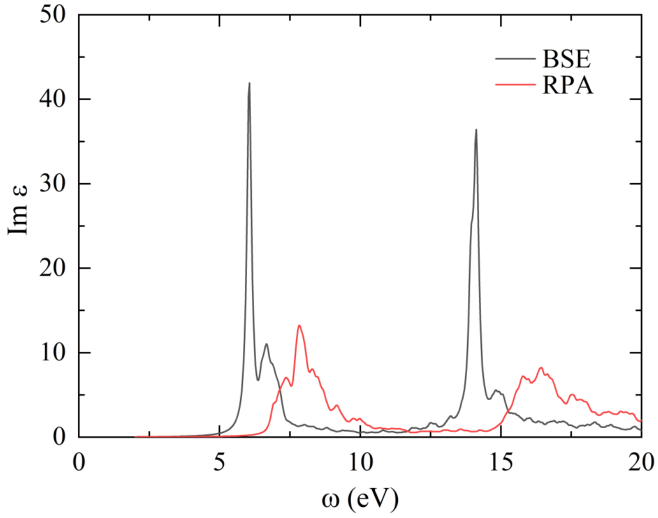


FIG. S1. The calculated imaginary parts of dielectric functions with BSE and RPA.

### B. The oscillator strength and the binding energy.

The imaginary part of the dielectric function and the oscillator strength from solving BSE are shown in Fig. S2. We determine the binding energy from the plot of oscillator strength, where 0.76 eV is the binding energy of the lowest bright exciton state.

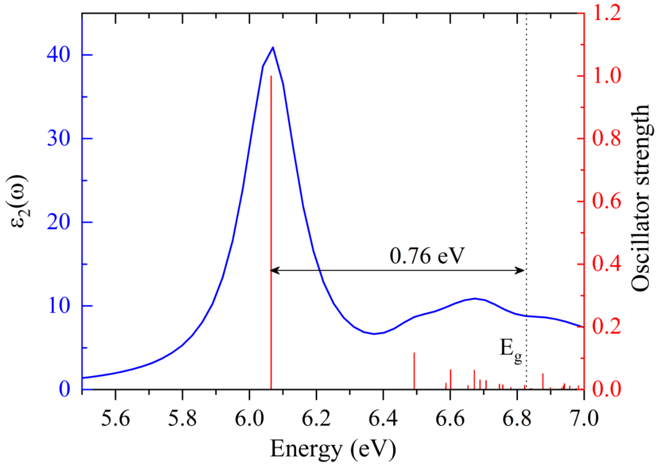


FIG. S2. The imaginary part of the dielectric function and the oscillator strength from solving BSE. The quasiparticle direct gap is 6.81 eV (the QE-LDA value plus a scissor of 2.314 eV).

## III. TEMPERATURE-DEPENDENT GENERALIZED ELIASHBERG FUNCTION

The temperature-dependent generalized Eliashberg function is given by

$$g^2F(\omega,T) = g^2F(\omega)(n(\omega,T)+1/2), \tag{2}$$

where $g^2F(\omega)$ is the generalized Eliashberg function given in figure 5 of the main text and $n(\omega,T)$ is the Bose factor. It is worth noting that the strength of the first two branches modes ZA and TA at low frequencies are enhanced which

is mainly responsible for the reduction of the band gap as the temperature increases. The $LO_3$ branch is mainly responsible for the reduction of the band gap with respect to the frozen-atom band gap.

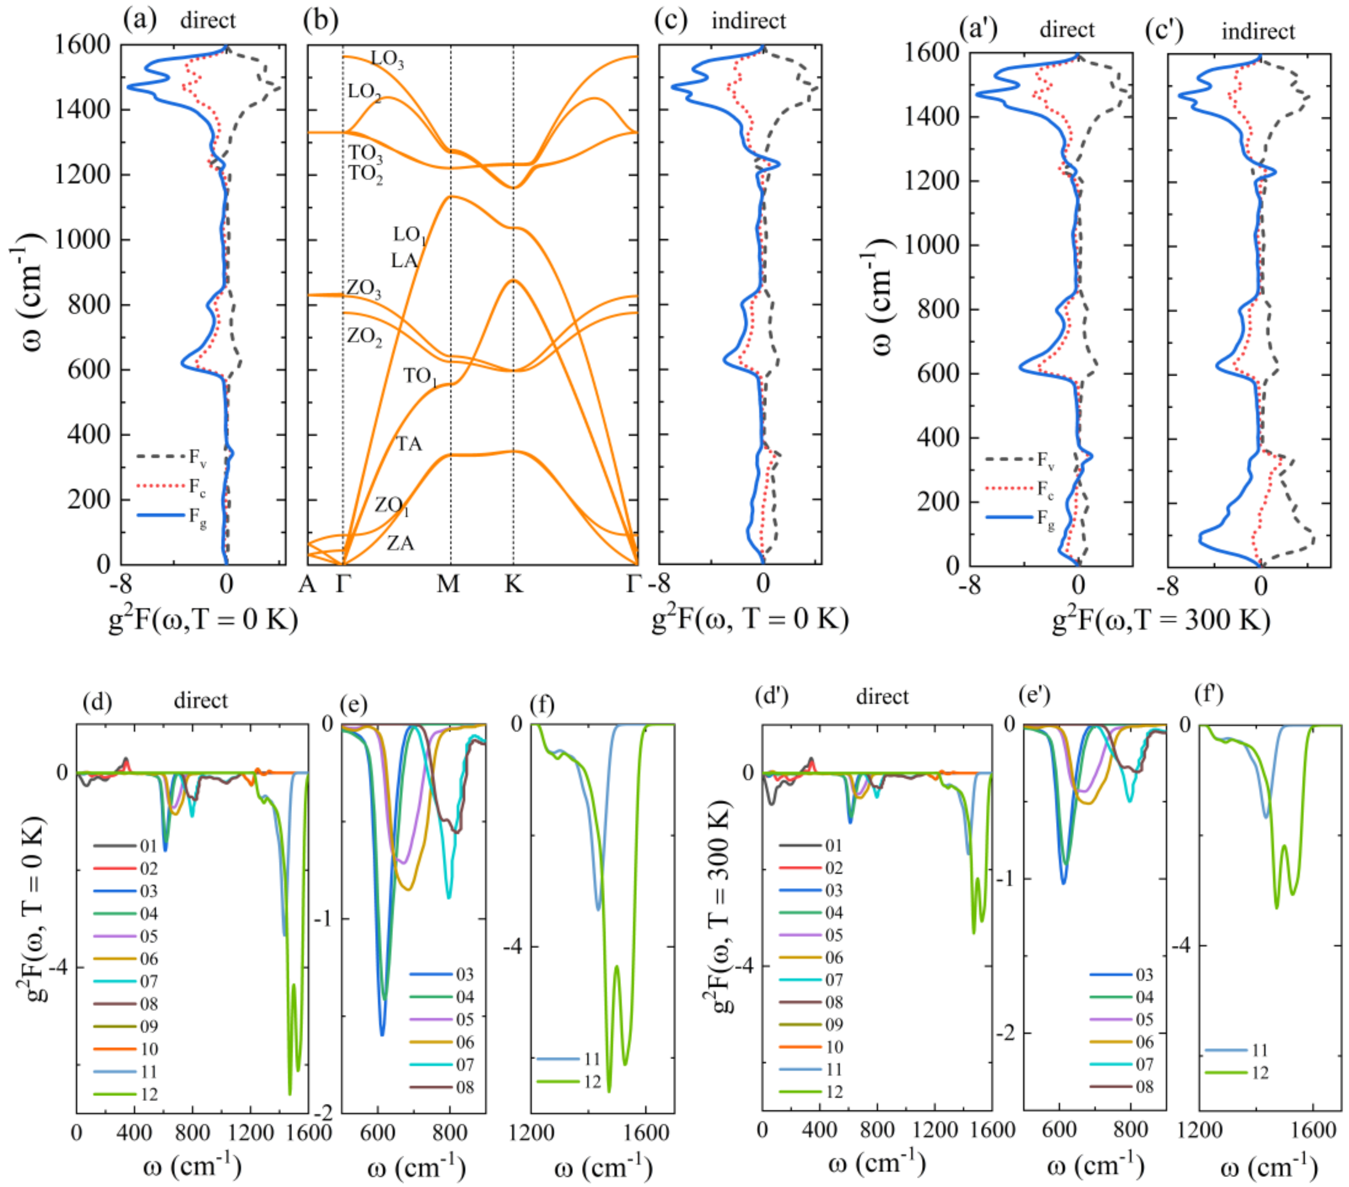


FIG. S3. The comparisons of temperature-dependent generalized Eliashberg functions $g^2F(\omega,T)$ between 0 K (a-f) and 300 K (a'-f').(a)Temperature-dependent generalized Eliashberg function for v (black dashed line), c (red dotted line), and band edge (blue solid line) of direct band gap at 0 K. (b) Phonon dispersion along selected symmetry points. (c) Temperature-dependent Eliashberg function of indirect band gap at 0 K. (d) The temperature-dependent direct band-edge Eliashberg function projected on each phonon modes. Only the most representative phonon modes are considered (e) below 900 $cm^{-1}$ and (f) above 1200 $cm^{-1}$.

## IV. CONVERGENCE TEST

### A. *GW* in the LAPW basis including HLOs

Concerning the HLOs, there are two main parameters: (i) additional number of nodes of the highest LOs with respect to the corresponding valence orbital as $n_{\rm LO}$, and (ii) the largest angular momentum $l^{\rm LO}_{\rm max} = l^{v}_{\rm max} + 1$, with $l^{v}_{\rm max}$ being the largest angular momentum of valence orbitals for each element. Figure S4 shows the convergence of the $G_0W_0$ band gap with respect to the number of additional high-energy local orbitals ($n_{\rm LO}$) and largest angular momentum ($l^{\rm LO}_{\rm max}$) in the $G_0W_0$ calculation. The band gap increases less than 50 meV when $n_{\rm LO}$ increases from 0 to 5, while it has a significantly increase with $l^{\rm LO}_{\rm max}$ increasing.

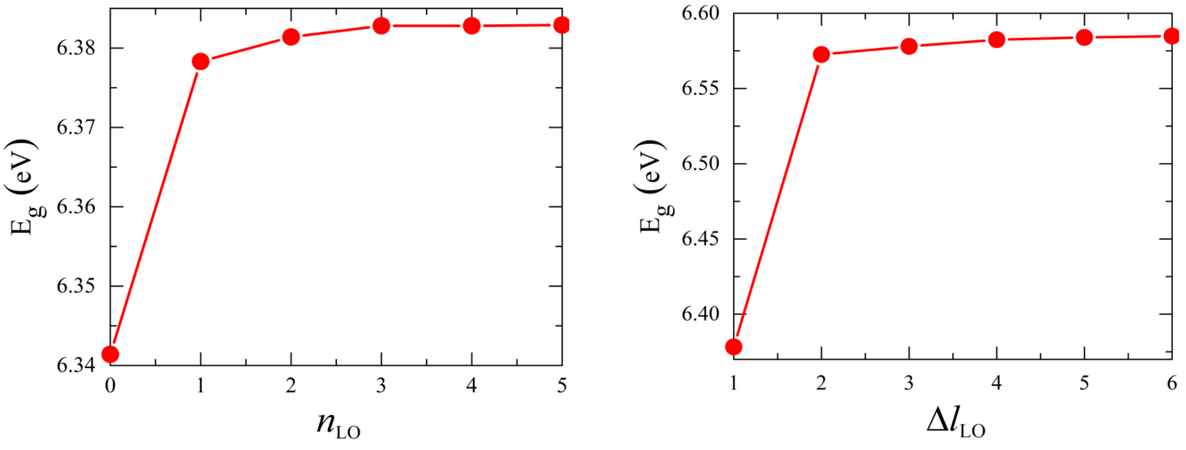


FIG. S4. Convergence of the $G_0W_0$@LDA band gap ($E_g$) of $h$-BN, calculated with $N_k = 2 \times 2 \times 1$ as a function of the number of additional high-energy local orbitals $n_{\rm LO}$ (left panels, with $l^{\rm LO}_{\rm max} = l^{\rm LO}_{\rm max}(def)$) and additional angular momentum $\Delta l_{\rm LO}$ in $l^{\rm LO}_{\rm max} = l^{v}_{\rm max} + \Delta l_{\rm LO}$ (right panels, with $n_{\rm LO} = 5$), respectively.

### B. Exciton and phonon coupling

The convergence tests of exciton and phonon coupling include k-grid (see Table S2), the number of electronic bands (see Fig. S5) and random q-points (see Fig. S6 and S7). The imaginary parts of the quasiparticle energies (represent the width of the spectrum) have small changes less than 30 meV of the position of the peak, which is negligible (see Fig. S7).

TABLE S2. The convergence test of the renormalizations of the indirect and direct band gaps in the unit of eV with respect to the k-grid at 0 K and 300 K, respectively. Using 200 bands and 50 random q-points and the errors of the real parts of the quasiparticle energies are less than 20 meV.

| | 0 K | | 300 K | |
|---|---|---|---|---|
| k-grid | direct | indirect | direct | indirect |
| $6 \times 6 \times 2$ | -0.178 | -0.210 | -0.195 | -0.270 |
| $9 \times 9 \times 2$ | -0.178 | -0.208 | -0.196 | -0.264 |

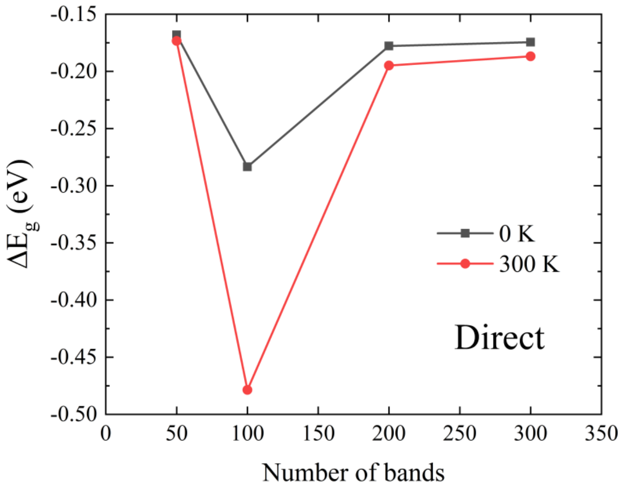


FIG. S5. The convergence test of the direct (left) and indirect (right) band gaps renormalization of $h$-BN as a function of the number of electronic bands at 0 K and 300 K, respectively. The number of random q-point is set as 50 and $6 \times 6 \times 2$ k-grid is used. Using 300 electronic bands is enough for band gaps, where the errors of the real parts of the quasiparticle energies of the number of bands are less than 30 meV.

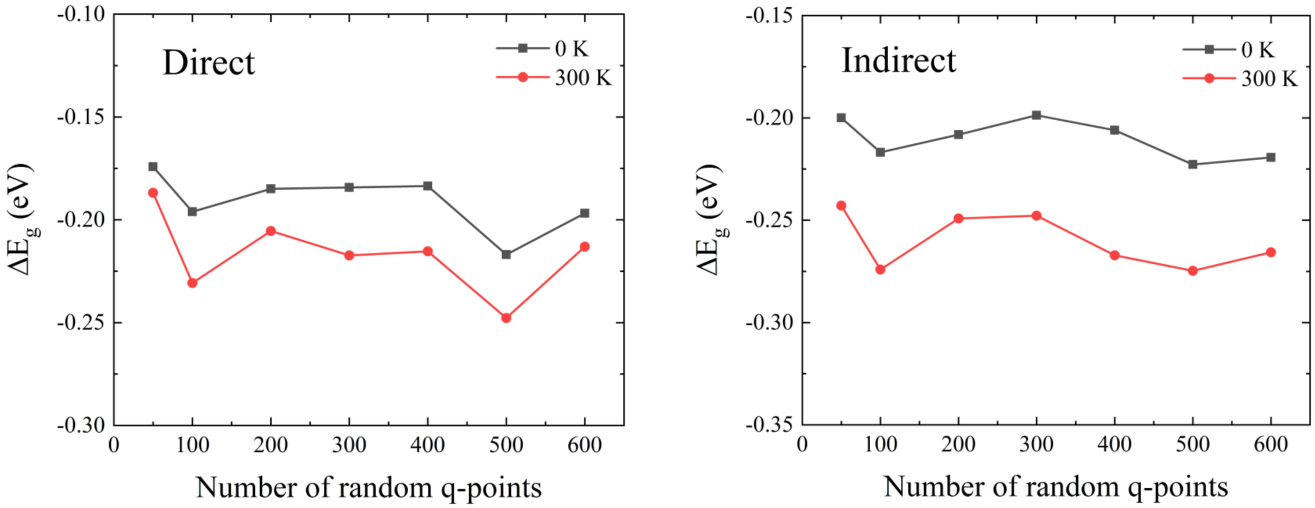


FIG. S6. The convergence test of the direct (left) and indirect (right) band gaps renormalization of $h$-BN as a function of the number of random q-points at 0 K and 300 K, respectively. The number of electronic bands is set as 300 and $6 \times 6 \times 2$ k-grid is used. Here, 600 random q-points is enough, where the errors of the real parts of the quasiparticle energies of random q-points are less than 30 meV.

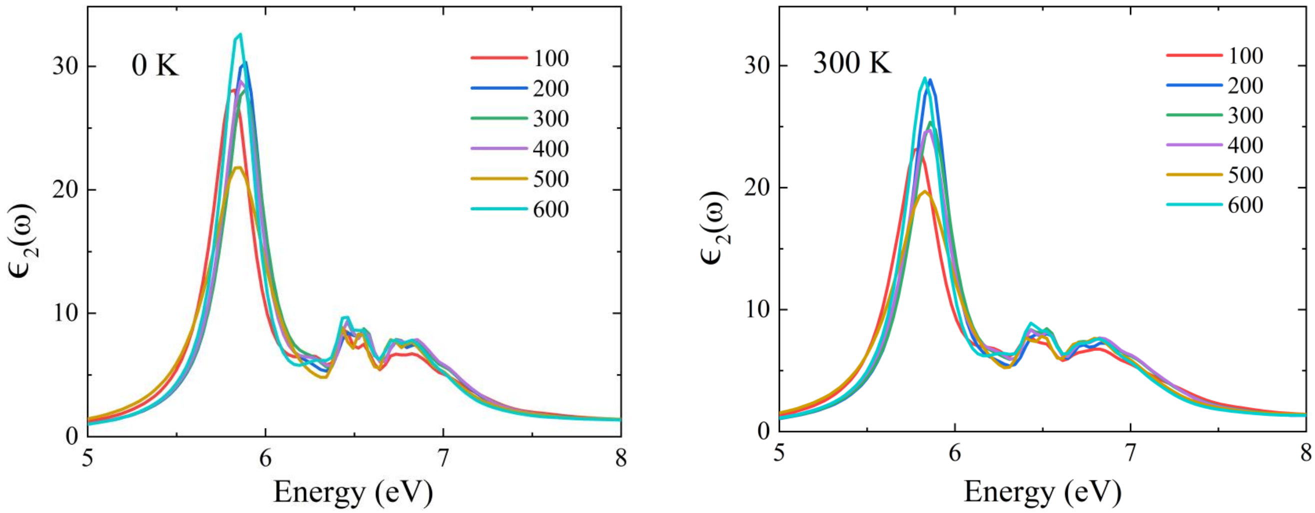


FIG. S7. The convergence test of the number of random q-points for the imaginary parts of the dielectric functions at 0 K (left) and 300 K (right) , respectively. The number of electronic bands is set as 300 and $6 \times 6 \times 2$ k-grid is used. The positions of the peak have small changes less than 30 meV.
